# Supplementary material for: Quantization and Semiclassics
Source: arXiv:1009.0444 source file (2010-09-01)
Supplement: Supplementary file 1 [file appendix.tex]

\begin{appendix}
	
\end{appendix}
