# Supplementary material for: Quantization and Semiclassics
Source: arXiv:1009.0444 source file (2010-09-01)
Supplement: Supplementary file 2 [file title.tex]

% \titlehead{
% \begin{center}
% \Huge
%  \\
% \end{center}
% } 

% \subject{Dissertation} 

\title{Weyl Quantization and Semiclassics}
\subtitle{Lecture Notes\\ {\small WS 2009/2010}}

\author{Max Lein\footnote{\texttt{lein@ma.tum.de}}}
\date{\today} 

\publishers{\vspace{20mm}
\includegraphics{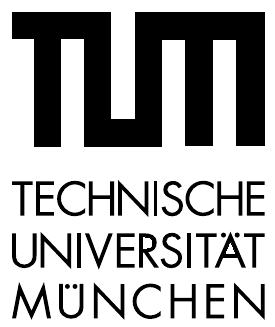} \\ 
Zentrum Mathematik \\
Lehrstuhl M5 \\
Boltzmannstr. 3 \\
85747 Garching 
}
