# Supplementary material for: Quantization and Semiclassics
Source: arXiv:1009.0444 source file (2010-09-01)
Supplement: Supplementary file 3 [file header.tex]

\documentclass[a4paper,10pt,pointlessnumbers,headtopline,headsepline]{scrbook}
\usepackage{usual_includes_Gentium}

\setcounter{tocdepth}{3}
\linespread{1.05}

%%% general definitions %%% (fold)

\providecommand{\FourierTrafo}{\mathfrak{F}}
\providecommand{\sympForm}{\sigma}
\providecommand{\Pspace}{\R^d_x \times \R^d_p}
\providecommand{\Cont}{\mathcal{C}}
\providecommand{\BCont}{\mathcal{BC}}
\providecommand{\Cpol}{\Cont_{\mathrm{pol}}}
\providecommand{\Fourier}{\FourierTrafo}
\providecommand{\spec}{\mathrm{spec} \, }
\providecommand{\image}{\mathrm{im} \, }
% \providecommand{}{}
% \providecommand{}{}
% \providecommand{}{}
% \providecommand{}{}

%%% end general definitions %%% (end)


%%% definitions chapter 1 %%% (fold)

\providecommand{\Op}{\mathfrak{Op}}
\providecommand{\OpA}{\Op^A}
\providecommand{\F}{\FourierTrafo}
\providecommand{\Fs}{\FourierTrafo_{\sympForm}}
\providecommand{\PA}{\mathsf{P}^A}
\providecommand{\Qe}{\mathsf{Q}}
\providecommand{\Pe}{\mathsf{P}}
\providecommand{\Weyl}{\sharp}
\providecommand{\magB}{\Weyl^B}
\providecommand{\magBel}{\magB_{\eps,\lambda}}
\providecommand{\Hoer}[1]{S^{#1}(\Pspace)}
\providecommand{\Hoerrd}[1]{S^{#1}_{\rho,\delta}(\Pspace)}
\providecommand{\Hoermrd}[3]{S^{#1}_{#2,#3}(\Pspace)}
\providecommand{\Hoerrdan}[1]{S^{#1}_{\rho,\delta}(\syspace)}
\providecommand{\Hoermrdan}[3]{S^{#1}_{#2,#3}(\syspace)}
\providecommand{\Hoeran}[1]{S^{#1}(\syspace)}
\providecommand{\wastlim}{{\mathrm{w}^{\ast}\mbox{-}\lim}}
\providecommand{\slim}{\mathrm{s}\mbox{-}\lim}
\providecommand{\WeylSys}{W}
\providecommand{\pspace}{\Xi}
% \providecommand{}{}
% \providecommand{}{}
% \providecommand{}{}
% \providecommand{}{}
% \providecommand{}{}
% \providecommand{}{}
% \providecommand{}{}
% \providecommand{}{}

%%% end definitions chapter 1 %%% (end)


%%% definitions chapter 2 %%% (fold)

% FIXME sort out superfluous definitions
\providecommand{\GA}{{\Gamma^A}}
\providecommand{\GAe}{{\Gamma^A_{\eps}}}
\providecommand{\GBe}{{\Gamma^B_{\eps}}}
\providecommand{\OBel}{{\Omega^B_{\eps,\lambda}}}
\providecommand{\GAe}{{\Gamma^A_{\eps}}}
\providecommand{\gBe}{{\gamma^B_{\eps}}}
\providecommand{\OBel}{\Omega^B_{\eps,\lambda}} 
\providecommand{\oBel}{\omega^B_{\eps,\lambda}} 

\providecommand{\spec}{\mathrm{spec}}

\providecommand{\PAc}{{\mathsf{p}^A_{c}}}
\providecommand{\PiAc}{{\mathsf{P}^A_{c}}}
\providecommand{\Qe}{{Q_{\eps}}}
\providecommand{\PiAel}{{\Pi^{A}_{\eps,\lambda}}}

\providecommand{\Hd}{H_{\mathrm{D}}}

\providecommand{\PSpace}{T^{\ast} \R^d}

\providecommand{\ordere}[1]{\mathcal{O}(\eps^{#1})}
\providecommand{\orderl}[1]{\mathcal{O}(\lambda^{#1})}
\providecommand{\orderone}{\mathcal{O}(1)}
\providecommand{\eprec}{\epsilon}
\providecommand{\ordereprec}{\mathcal{O}(\eprec +)}

\providecommand{\order}{\mathcal{O}} 
\providecommand{\orderc}[1]{\mathcal{O}(\nicefrac{1}{c^{#1}})}

\providecommand{\Piref}{\hat{\Pi}_{\mathrm{ref}}}
\providecommand{\piref}{\pi_{\mathrm{ref}}}

\providecommand{\Hfast}{\mathcal{H}_{\mathrm{fast}}}
\providecommand{\Hslow}{\mathcal{H}_{\mathrm{slow}}}
\providecommand{\Hphys}{\mathcal{H}_{\mathrm{phys}}}

\providecommand{\Fs}{\mathcal{F}_{\sigma}}

\providecommand{\Weyl}{\star}
\providecommand{\Weyle}{\Weyl_{\eps}}
\providecommand{\magB}{\sharp^B}
\providecommand{\magBe}{\Weyle^B}
\providecommand{\magBl}{\Weyl^B_{\lambda}}
\providecommand{\magBel}{\Weyl^B_{\eps,\lambda}}
\providecommand{\magBc}{\sharp^B_c}

\providecommand{\Ael}{A^{\eps,\lambda}}
\providecommand{\Bel}{B^{\eps,\lambda}}
\providecommand{\Bte}{\tilde{B}^{\eps}}

\providecommand{\Opel}{\mathrm{Op}_{\eps,\lambda}}
\providecommand{\OpAsr}{\mathrm{Op}^A_c} 
\providecommand{\Op}{\mathrm{Op}}
\providecommand{\OpAus}{\Op^A_{\mathrm{u}}}
\providecommand{\OpAel}{\mathrm{Op}^A_{\eps,\lambda}}
\providecommand{\Ope}{\mathrm{Op}_{\eps}}

\providecommand{\WeylSysAel}{{W^A_{\eps,\lambda}}}
\providecommand{\WeylUs}{W^A_{\mathrm{u}}}
\providecommand{\WeylSysA}{W^A}

\providecommand{\WignerTrafoel}{{\mathcal{W}^A_{\eps,\lambda}}}
\providecommand{\WignerTrafo}{{\mathcal{W}}}
\providecommand{\WignerUs}{\tilde{\mathcal{W}}^A}

\providecommand{\minsAl}{\vartheta^A_{\lambda}}

% TODO fix notational clash
\providecommand{\Hoer}[1]{\mathcal{S}^{#1}}
% \providecommand{\Hoerrd}[1]{\mathcal{S}^{#1}_{\rho,\delta}}
% \providecommand{\Hoermrd}[3]{\mathcal{S}^{#1}_{#2,#3}}
\providecommand{\SemiHoer}[1]{\mathrm{A}\Hoer{#1}}
\providecommand{\SemiHoerrd}[1]{\mathrm{A}\Hoerrd{#1}}
\providecommand{\SemiHoermrd}[3]{\mathrm{A}\Hoermrd{#1}{#2}{#3}}
\providecommand{\PsiHoer}[1]{\Psi\Hoerrd{#1}}
\providecommand{\Schwartz}{\mathcal{S}}

\providecommand{\Href}{\mathcal{H}_{\mathrm{ref}}}
\providecommand{\rel}{\mathrm{rel}}
% \providecommand{}{}
% \providecommand{}{}
% \providecommand{}{}
% \providecommand{}{}
% \providecommand{}{}
% \providecommand{}{}
% \providecommand{}{}
% \providecommand{}{}
% \providecommand{}{}
% \providecommand{}{}
% \providecommand{}{}
% \providecommand{}{}
% \providecommand{}{}
% \providecommand{}{}
% \providecommand{}{}
% \providecommand{}{}
% \providecommand{}{}
% \providecommand{}{}

%%% end definitions chapter 2 %%% (end)


%%% definitions chapter 3 %%% (fold) 

% \providecommand{}{}
% \providecommand{}{}
% \providecommand{}{}
% \providecommand{}{}
% \providecommand{}{}
% \providecommand{}{}
% \providecommand{}{}
% \providecommand{}{}
% \providecommand{}{}
% \providecommand{}{}
% \providecommand{}{}
% \providecommand{}{}
% \providecommand{}{}
% \providecommand{}{}
% \providecommand{}{}
% \providecommand{}{}
% \providecommand{}{}
% \providecommand{}{}
% \providecommand{}{}

%%% end definitions chapter 3 %%% (end) 


%%% definitions chapter 4 %%% (fold) 

% \providecommand{}{}
% \providecommand{}{}
% \providecommand{}{}
% \providecommand{}{}
% \providecommand{}{}
% \providecommand{}{}
% \providecommand{}{}
% \providecommand{}{}
% \providecommand{}{}
% \providecommand{}{}
% \providecommand{}{}
% \providecommand{}{}
% \providecommand{}{}
% \providecommand{}{}
% \providecommand{}{}
% \providecommand{}{}
% \providecommand{}{}
% \providecommand{}{}
% \providecommand{}{}

%%% end definitions chapter 4 %%% (end) 


% TODO clean up TeX commands (products in particular)
%%% definitions chapter 5 %%% (fold) 
\providecommand{\Rep}{\mathfrak{Rep}} 
\providecommand{\repcom}{\star}
\providecommand{\reptau}{\repcom_{\theta,\tau}}
\providecommand{\repom}{\repcom^{\omega}_{\theta,\tau}}

\providecommand{\Xgroup}{\mathcal{X}}
\providecommand{\AB}{\mathfrak{A}^B}
\providecommand{\Alg}{\mathcal{A}}
\providecommand{\Hil}{\mathcal{H}}
\providecommand{\Xalg}{\Xgroup,\Alg}
\providecommand{\CA}{\mathfrak{C}_{\Alg}}
\providecommand{\CBA}{\CA^B}
\providecommand{\Unit}{\mathcal{U}}
\providecommand{\Ralg}{{\R^d};\Alg}
\providecommand{\syspace}{{\R^d}^*;\Alg^{\infty}}
% \providecommand{\syspace}{\Xgroup^*;\Alg^{\infty}}
\providecommand{\BBA}{\mathfrak{B}^B_{\Alg}}
\providecommand{\CBA}{\mathfrak{C}^B_{\Alg}}
\providecommand{\MBA}{\mathfrak{M}^B_{\Alg}}
\providecommand{\Salg}{\mathcal{S}_{\Alg}}
\providecommand{\SalgComp}{F_{\Alg}}
\providecommand{\Quasi}{\mathsf{Q}}
\providecommand{\oB}{\omega^B}
\providecommand{\WeylSyslt}{W^{\lambda}_{\tau}}

\providecommand{\Aut}{\mathrm{Aut}}
\providecommand{\dualX}{\hat{\Xgroup}}
\providecommand{\Xprod}{\Alg \rtimes_{\theta,\tau} \Xgroup}
\providecommand{\sXprod}{\mathfrak{C}_{\Alg}}
\providecommand{\twistedXprod}{\Alg \rtimes_{\theta,\tau}^{\omega} \Xgroup}
\providecommand{\stwistedXprod}{\sXprod^{\omega}}
\providecommand{\Ideal}{\mathcal{I}}
% FIXME notation not ideal
\providecommand{\sFXprod}{\Fourier \mathfrak{C}^{\omega}_{\Alg}}
% \providecommand{}{}
% \providecommand{}{}
% \providecommand{}{}
% \providecommand{}{}
% \providecommand{}{}
% \providecommand{}{}
% \providecommand{}{}
% \providecommand{}{}
% \providecommand{}{}
% \providecommand{}{}
% \providecommand{}{}

%%% end definitions chapter 5 %%% (end) 



%%% definitions chapter 6 %%% (fold) 

\providecommand{\crossB}{\repcom^B_{\theta}}
\providecommand{\mult}{\mathcal{M}}
\providecommand{\fxb}{\mathfrak{B}^B_{\Alg}}
\providecommand{\BopL}{\mathcal{B} \bigl ( L^2(\R^d) \bigr )}
\providecommand{\Calg}{\mathfrak{C}}
\providecommand{\Index}{\mathcal{J}}
% \providecommand{}{}
% \providecommand{}{}
% \providecommand{}{}
% \providecommand{}{}
% \providecommand{}{}
% \providecommand{}{}
% \providecommand{}{}
% \providecommand{}{}
% \providecommand{}{}
% \providecommand{}{}
% \providecommand{}{}
% \providecommand{}{}
% \providecommand{}{}
% \providecommand{}{}
% \providecommand{}{}

%%% end definitions chapter 6 %%% (end) 







\providecommand{\opHBO}{\hat{H}_{\mathrm{BO}}}
\providecommand{\HBO}{{H}_{\mathrm{BO}}}
\providecommand{\He}{H_{\mathrm{e}}}
% \providecommand{}{}
% \providecommand{}{}
% \providecommand{}{}
% \providecommand{}{}
% \providecommand{}{}
% \providecommand{}{}
% \providecommand{}{}
% \providecommand{}{}
% \providecommand{}{}
% \providecommand{}{}
% \providecommand{}{}
% \providecommand{}{}
% \providecommand{}{}
% \providecommand{}{}
% \providecommand{}{}
% \providecommand{}{}
% \providecommand{}{}
% \providecommand{}{}
